# Supplementary material for: Forecasting People Trajectories and Head Poses by Jointly Reasoning on Tracklets and Vislets
Source: arXiv:1901.02000 source file (2019-10-15)
Supplement: Supplementary file 1 [file suppmaterial_text.tex]

This supplementary material provides additional qualitative results, more details on some of the paper equations, more information on the adopted code and errata to the paper.

Please watch the attached {\tt supmat.mp4} for more qualitative results. In particular, the video illustrates the the role that vislets play in the MX-LSTM.

Additionally, this pdf provides the following:
%In this supplementary material we provide new qualitative results, details omitted in the main text, and we fix a sentence which may rise misunderstandings.
\begin{itemize}
    %\item The video file {\tt xxx.avi} gives qualitative results in addition to those reported in the paper;
    \item Sec.~\ref{sec:ablation} gives the equations for the ablation models;
    \item Sec.~\ref{sec:implementation} details the implementation of the MX-LSTM;
    \item Sec.~\ref{sec:code} provides the http addresses of the code used for the comparative experiments;
    \item Sec.~\ref{sec:errata} revises a sentence in the paper, expressing it in a clearer way.
\end{itemize}

\section{Ablation study: equations}\label{sec:ablation}
On rows 623-630 we introduced the \textbf{Block-Diagonal MX-LSTM (BD-MX-LSTM)}: The equations that differ w.r.t. MX-LSTM's Eq. (7) and (9) are, respectively, 
\begin{eqnarray}
L^i(\mathbf{W}_{x},\mathbf{W}_{a},\mathbf{W}_H,\mathbf{W}_{\text{LSTM}},\mathbf{W}_{o}) &=&\nonumber\\  -\sum_{T_{obs}+1}^{T_{pred}}log\left( P([\mathbf{x}^{(i)}_t]^T|\bo{\mu}^{(x,i)}_t,\bo{\sigma}^{(x,i)}_t,\rho^{(x,i)}_t \right)+\!\!\\\nonumber
log\left(P([\mathbf{a}^{(i)}_t]^T|\bo{\mu}^{(a,i)}_t,\bo{\sigma}^{(a,i)}_t,\rho^{(a,i)}_t\right)
\end{eqnarray}
where $\bo{\mu}^{(x,i)}_t=[{}_x\mu^{(x,i)}_t,{}_y\mu^{(x,i)}_t]$ and ${}_x\mu^{(x,i)}_t$ is the x-component of $\bo{\mu}$ and the same applies for the standard deviation vector $\bo{\sigma}^{(x,i)}_t$.

The second log term of (1) represents the likelihood's fit for the anchor points of the vislets.
Equation (9) in the main paper becomes:
\begin{equation}
[\bo{\mu}^{(x,i)}_t,\bo{\sigma}^{(x,i)}_t,\rho^{(x,i)}_t,\bo{\mu}^{(a,i)}_t,\bo{\sigma}^{(a,i)}_t,\rho^{(a,i)}_t]^T \!=\! \mathbf{W}_o \mathbf{h}^{(i)}_{t-1}\label{eq:params}
\end{equation}
 
\section{Implementation details} \label{sec:implementation}

For training MX-LSTM and the ablation study models, we use a learning rate of 0.005 along with the RMS-prop optimizer. We set the embedding dimension for spatial coordinates and vislets to 64 and the hidden state dimension is $D=128$.
We plan to release the code upon acceptance.

\section{Code used for the experiments} \label{sec:code}
\begin{itemize}
    \item Social Force Model (SF)~\cite{yamaguchi2011cvpr}: code received from the authors (in particular, {\tt kyamagu@vision.is.tohoku.ac.jp}) 
    \item Linear Trajectory Avoidance (LTA)~\cite{pellegrini2009iccv}: code received by {\tt kyamagu@vision.is.tohoku.ac.jp}
    \item Vanilla LSTM and Social LSTM (S-LSTM)~\cite{alahi2016cvpr} \url{https://web.stanford.edu/~alahi/index.html#code} 
\end{itemize}

\section{Errata} \label{sec:errata}

Starting from row 742:

``If we provide to MX-LSTM an artificial observation sequence with \textbf{no 
trajectory} but vislets oriented toward west (third column, orange 
arrows), where no people are present, the MX-LSTM predicts a trajectory 
departing from the group (cyan trajectory and arrows).''\\

The sentence above should instead have read:\\

``If we provide to MX-LSTM an artificial observation sequence with \textbf{the annotated positions (\ie the real trajectory)} but vislets oriented toward west (third column, orange arrows), where no people are present, the MX-LSTM predicts a 
trajectory departing from the group (cyan trajectory and arrows).''\\

%%% Fabio's version:
%``If we provide MX-LSTM with a fictitious observation sequence with the real positions (\ie the real trajectory) but vislets oriented toward west (third column, orange arrows), pointing to an opposite direction from the group of people, the MX-LSTM predicts a trajectory departing from the group (cyan trajectory and arrows).''\\

%The misplaced original sentence was due to the fact that the GT trajectory was essentially a point, since the pedestrian is static.
